# Supplementary material for: OTClean: Data Cleaning for Conditional Independence Violations using Optimal Transport
Source: arXiv:2403.02372 source file (2024-03-04)
Supplement: Supplementary file 1 [file appendix.tex]

\section{Proofs and Additional Propositions}\label{sec:proofs}

\subsection{Reducing the Unsaturated CI Repair problem to Saturated}\label{sec:unsat}

We first define candidates for $\pi$, denoted by $\pi^*$, and describe its relationship with $\pi_\sigma$.

\begin{definition} \label{df:reduce} Consider a probability function $p$ with random variables $\st{V}=\{X,Y,W\}$, a cost function $c$ based on Euclidean distance, and an unsaturated CI constraint $\sigma:X\indep Y$. A coupling $\pi^*$ is a joint probability function over two sets of random variables $\st{V}=\{X,Y,W\}$, and $\st{V}'=\{X',Y',W'\}$ that satisfies the following:
\begin{itemize}
    \item $\pi^*_{X,Y,X',Y'}=\pi_\sigma$.
    \item $\pi^*_{X,Y,W}=p$.
    \item For every $w_i,w_j\in \dom{W}$, if $w_i\neq w_j$ then $\pi^*_{W,W'}(w,w')=0$. 
\end{itemize}

\noindent We denote $\pi^*_{X',Y',W'}$ (the marginal of $\pi^*$ w.r.t. $X,Y$) by $p^*$.\boxtheorem
\end{definition}

%The first property in Definition~\ref{df:reduce} means the marginal of $\pi^*$ w.r.t. the variables in $\sigma$ (i.e., $X,Y,W$ and $X',Y',W'$) is $\pi_\sigma$. The second property required the marginal of $\pi^*$ w.r.t. $X,Y,W$ to be $p$. The last property means the marginal of $\pi^*$ w.r.t. $W,W'$ is the identity coupling.

%Note that we assumed $\pi^*$ is a joint probability function on $X,Y,W$ as source random variables and $X',Y',W'$ as the destination random variables, where the source of the destination variables share domains. 

\begin{proposition} \label{pr:optimal} The probability distribution function $q^*$ in Definition~\ref{df:reduce} is an optimal repaired distribution function.\boxtheorem 
\end{proposition}

{\em Proof sketch:} The probability function $q^*$ is a repair (satisfies $\sigma$) since its marginal is $q_\sigma$ (due to the first property) and $q_\sigma$ satisfies $\sigma$ by definition. $q^*$ is also optimal because it has the minimum distance with $p$. This is guaranteed by the second and the third properties; the second property ensures the minimum distance is computed w.r.t. $p$, and the third property guarantees that there is no unnecessary mass transport between different values of $W$, which means all the mass transport is essential for satisfying $\sigma$. \boxtheorem  

We use Proposition~\ref{pr:optimal} to design an algorithm to efficiently find a possible function $\pi^*$. Note $\pi^*$ is not necessarily unique (see Appendix~\ref{sec:problem} for an example). Algorithm~\ref{alg:coupling} shows the detail of this algorithm. We first present Example~\ref{ex:building} that explains $p^*$ and $\pi^*$ and later use it to describe Algorithm~\ref{alg:coupling}.

\begin{example} \label{ex:building} Consider a probability function $p(\vt{v})$ with random variables $\st{V}=\{X,Y,W\}$ and the domain sets $\dom{X}=\dom{Y}=\dom{W}=\{0,1\}$. Let $p$ assign the following probabilities to values in $\dom{V}$ (we always omit values with zero probabilities for brevity): 
\begin{align*}
(0,0,0)\mapsto 0.1,\;\;\;(1,1,0)\mapsto 0.1,\;\;\;
(0,0,1)\mapsto 0.4,\;\;\;(1,1,1)\mapsto 0.4.  
\end{align*}

\noindent The function $p$ has the marginal probability function $p_{X,Y}$ with the probabilities $(0,0)\mapsto 0.5,(1,1)\mapsto 0.5$. Both $p$ and $p_{X,Y}$ violate $\sigma:X\indep Y$, i.e., $p\not\models \sigma$ and $p_{X,Y}\not\models \sigma$, and an optimal repair of $p_\sigma=p_{X,Y}$ w.r.t. the saturated constraint $\sigma$ is $q_\sigma=\{(0,0)\mapsto 0.25,(1,1)\mapsto 0.25,(0,1)\mapsto 0.25,(1,0)\mapsto 0.25\}$ which can be obtained from a coupling $\pi_\sigma$ with the following probabilities: 
\begin{align*}
(0,0,0,0)\mapsto 0.25,\;\;\;(0,0,0,1)\mapsto 0.25,\\
(1,1,1,1)\mapsto 0.25,\;\;\;(1,1,1,0)\mapsto 0.25.  
\end{align*}

\noindent The coupling $\pi_\sigma$ generates $q_\sigma$ by transporting $0.25$ mass from $(0,0)$ to $(0,1)$ and the same amount from $(1,1)$ to $(1,0)$. 

A coupling $\pi^*$ has the following probabilities:
\begin{align*}
(0,0,\underline{0},0,0,\underline{0})\mapsto 0.1,&\;\;\;(1,1,\underline{0},1,1,\underline{0})\mapsto 0.1,\\
(0,0,\underline{1},0,0,\underline{1})\mapsto 0.15,&\;\;\;(0,0,\underline{1},0,1,\underline{1})\mapsto 0.25,\\
(1,1,\underline{1},1,1,\underline{1})\mapsto 0.15,&\;\;\;(1,1,\underline{1},1,0,\underline{1})\mapsto 0.25.
\end{align*}

\noindent $\pi^*$ generates a repair $q^*$ with the probabilities\begin{align*}
(0,0,0)\mapsto 0.1,&\;\;\;(1,1,0)\mapsto 0.1,\;\;\;\\
(0,0,1)\mapsto 0.15,&\;\;\;(1,1,1)\mapsto 0.15,\\  
(0,1,1)\mapsto 0.25,&\;\;\;(1,0,1)\mapsto 0.25. 
\end{align*}

\noindent $q^*$ is an optimal repair with the minimum distance with $p$.

$\pi^*$ satisfies the three properties in Definition~\ref{df:reduce}. In particular, it has the last property as the underlined values of $W$ above do not change for each non-zero probability which means masses are not transported between different values of $W$, and all the mass transport is to satisfy $\sigma$ as in $\pi_\sigma$.\boxtheorem \end{example}

The idea of Algorithm~\ref{alg:coupling} is to build $\pi^*$ by transporting mass from $\st{V}=X,Y,Z$ to $\st{V}'=\{X',Y',Z'\}$ as instructed by $\pi_\sigma$ while making all the mass transport is from the same vales of $W$ and $W'$. Running the algorithm with our running example in Exmaple~\ref{ex:building}, it starts with $(0,0)$ in Line 2 and initialize $\vt{s}$ with $[0.1,0.4]$ in Line 3 as $p_{W|X,Y}(0|0,0)=0.1$ and $p_{W|X,Y}(1|0,0)=0.4$. Then, in Lines 5-16, the algorithm transports the masses in $\vt{s}$ according to $\pi_\sigma$. In Line 7, it starts with mapping from $(0,0)$ to $(0,0)$ and initialize $d=0.25$ in Line 6 since $\pi_\sigma(0,0,0,0)=0.25$. The algorithm continues with Lines 7-16, where it first transports $\vt{s}[0]=0.1$ from $(0,0,0)$ to $(0,0,0)$ and updates the remaining probability to $d=0.15$. It also updates $\delta=0.1$ and $c=1$ in Lines 9-11, and $\mathcal{M}((0,0,0),(0,0,0))=\delta=0.1$ in Lines~16 and 17. It continues the while loop transporting mass from $(0,0,1)$ to $(0,0,1)$, but this time updates $\vt{s}[1]=0.4-0.15=0.25$, $\delta=0.15$, and $d=0$ in Lines~12-15, and then updates $\mathcal{M}((0,0,1),(0,0,1))=\delta=0.15$ in Lines~16 and 17. This completes transporting the mass $0.25$ from $(0,0)$ to $(0,0)$, and the algorithm continues the for loop in Line~5 for moving mass from $(0,0)$ to $(0,1)$. 

In the next iteration, $d=0.25$, and the algorithms starts with transporting mass from $(0,0)$ to $(0,1)$. Since $c=1$, it continues with transporting $\vt{s}[1]=0.25$ from $(0,0,1)$ to $(0,1,1)$. It updates $\vt{s}[1]=0$, $d=0$, and $\delta=0.25$ in Lines~13-15, and $\mathcal{M}((0,0,1),(0,1,1))=\delta=0.25$ in Lines~16 and 17. The algorithm continues until generating the coupling $\pi$ in Example~\ref{ex:building}.

\begin{algorithm}
\caption{$\textit{BuildCoupling}$}\label{alg:coupling}
\KwInput{A probability function $p$ and a coupling $\pi_\sigma$}
\KwOutput{A coupling $\pi$}
$\textit{Init}(\mathcal{M})$ \nComment{Initialize the probability mapping $\mathcal{M}$}\\
    \For{$(x_i,y_j) \in \dom{X}\times\dom{Y}$\label{ln:block-start}}{
    \lFor{$w_k\in\dom{W}$}{$\vt{s}[k] \leftarrow p_{W|X,Y}(w_k|x_i,y_i)$}
    $c\leftarrow 0;$\\
    \For{$(x'_i,y'_j) \in \dom{X}\times\dom{Y}$}{
         $d\leftarrow \pi_\sigma(x_i,y_i,x'_i,y'_i);$\\
         \While{d>0}{
                \If{$d > \vt{s}[c]$}{
                    $d \leftarrow d - \vt{s}[c];$\\
                    $\delta \leftarrow \vt{s}[c];$\\
                    $c \leftarrow c+1$;
                } \Else{
                    $\vt{s}[c] \leftarrow \vt{s}[c] - d;$\\
                    $\delta \leftarrow d;$\\
                   $d\leftarrow 0;$
                }
                $m\leftarrow \mathcal{M}[(x_i,y_i,w_c),(x'_i,y'_i,w_c)];$\\
                $\mathcal{M}[(x_i,y_i,w_c),(x'_i,y'_i,w_c)] \leftarrow  m+\delta$;
            }
        }
    } 
\Return{$\textit{pmf}(\mathcal{M});$}
\end{algorithm}

Wasserstein distance is the only distance function that has this nice property. It is shown in this section that in the case of solving the problem using KL divergence, repairing on marginal probability distribution is not equivalent with repairing on the complete distribution.
Assuming a dataset with three binary attributes X, Y, and W is given. we want to enforce $\sigma:X\indep Y$. Here is the vector representation of the empirical probability distribution of given dataset: (indexing is done using idx function)
$$\sourceM = [0.1,0,0,0.1,0.4,0,0,0.4] = $$
$$\begin{bmatrix}
0.1 & 0\\
0 & 0.1
\end{bmatrix}
\begin{bmatrix}
0.4 & 0\\
0 & 0.4
\end{bmatrix}$$
Its marginal probability distribution on X and Y is as follows:
$$\sourceM_{X,Y} = [0.5,0,0,0.5] = $$
$$\begin{bmatrix}
0.5 & 0\\
0 & 0.5
\end{bmatrix}$$
if we solve an optimization problem that finds a repaired probability distribution which satisfies our CI constraint and minimizes KL divergence instead of Wasserstein distance, the result would be a uniform probability distribution:
$$q_{X,Y} = [0.25,0.25,0.25,0.25] = $$
$$\begin{bmatrix}
0.25 & 0.25\\
0.25 & 0.25
\end{bmatrix}$$
Now we show that deciding about the $q_{W|X,Y}$ is not arbitrary. As proved in the previous section, when minimizing Wasserstein distance, if the optimal mapping suggests moving mass m from (x,y) to (x',y'), it doesn't matter if we move this mass from (x,y,w) to (x',y',w) or from (x,y,w') to (x',y',w'). Here we show that it's not true when minimizing KL divergence. For converting $\sourceM_{X,Y}$ to $q_{X,Y}$, the mapping returned by optimal transport tells us that 0.25 mass must be transported from (0,0) to (0,1) and 0.25 mass must be transported from (1,1) to (1,0). we consider two coupling $\pi_1$ and $\pi_2$ for mapping $\sourceM$ to q; They build distributions $q_1$ and $q_2$ that their marginal on X and Y is $q_{X,Y}$ but $q_{1_{W|X,Y}}$ differs from $q_{2_{W|X,Y}}$.
$$\pi_{1_{(5,7)}}=0.25, \pi_{1_{(8,6)}}=0.25$$
$$\pi_{2_{(5,7)}}=0.15, \pi_{2_{(8,6)}}=0.15,\pi_{2_{(1,3)}}=0.1, \pi_{2_{(4,2)}}=0.1$$
$$q_1 = [0.1,0,0,0.1,0.15,0.25,0.25,0.15] = $$
$$\begin{bmatrix}
0.1 & 0\\
0 & 0.1
\end{bmatrix}
\begin{bmatrix}
0.15 & 0.25\\
0.25 & 0.15
\end{bmatrix}$$
$$q_2 = [0,0.1,0.1,0,0.25,0.15,0.15,0.25] = $$
$$\begin{bmatrix}
0 & 0.1\\
0.1 & 0
\end{bmatrix}
\begin{bmatrix}
0.25 & 0.15\\
0.15 & 0.25
\end{bmatrix}$$
The KL divergence between these repaired distributions and initial distribution is different. ($KL(\sourceM,q_1)=0.284, KL(\sourceM,q_2)=0.076$) So we don't have a algorithmic way to extend the marginal repair ($q_{X,Y}$) to build final unsaturated distribution ($q$).
